# Supplementary material for: Spatio-Temporal Distortion Aware Omnidirectional Video Super-Resolution
Source: arXiv:2410.11506 source file (2025-08-05)
Supplement: Supplementary file 1 [file AAAI2026_ICCV_Appendix_arXiv.pdf]

# Spatio-Temporal Distortion Aware Omnidirectional Video Super-Resolution Technical Appendix

**Hongyu An[1], Xinfeng Zhang[1*], Shijie Zhao[2], Li Zhang[2], Ruiqin Xiong[3]**

[1]University of Chinese Academy of Sciences, [1]Bytedance Inc, [1]Peking University
anhongyu22@mails.ucas.ac.cn, xfzhang@ucas.ac.cn,
{zhaoshijie.0526, lizhang.idm}@bytedance.com, rqxiong@pku.edu.cn

Due to the lack of space in the main paper, we provide more details of the proposed Spatio-Temporal Distortion Aware Network (STDAN) in the supplementary material. In Section 1, we present the Equirectangular Projection (ERP) transformation relationships from 3D sphere to 2D plane and the formula derivation of the projection distortion quantization. More experimental results and visual comparisons can be found in Section 2.

## 1. Equirectangular Projection

In this section, we follow the coordinate representation in the main paper and provide a rigorous derivation of the ERP and its associated distortion analysis. More precisely, spherical coordinates are defined as $(\rho, \theta, \phi)$, where $\theta \in (0, 2\pi)$ and $\phi \in (0, \pi)$ denote longitude and latitude, respectively. The corresponding planar horizontal and vertical coordinates are parameterized as $(u, v)$.

**1.1 Geometric Transformation** The coordinate transformation between 3D sphere and 2D plane is defined as:

$$\begin{cases} \rho = \sqrt{x^2+y^2+z^2}, \\ \theta = \arctan(y/x), \\ \phi = \arcsin(z/\rho). \end{cases} \begin{cases} x = \rho\cos(\phi)\cos(\theta), \\ y = \rho\cos(\phi)\sin(\theta), \\ z = \rho\sin(\phi). \end{cases} \tag{1}$$

$$\begin{cases} \theta = (u/W - 0.5)2\pi, \\ \phi = (0.5 - v/H)\pi. \end{cases} \begin{cases} u = (\theta/2\pi + 0.5)W, \\ v = (0.5 - \phi/\pi)H. \end{cases} \tag{2}$$

where ($x$, $y$, $z$) are world coordinates responding to spherical coordinates $(\rho, \theta, \phi)$, $H$ and $W$ indicate the height and width (in pixels) of the ERP omnidirectional image (ODI). Fig. 1 provides an illustrative example of the forward ERP projection and its exact inverse back-projection between the spherical and planar domains.

**1.2 Projection Distortion** Inspired by (Sun, Lu, and Yu 2017), we quantify the projection distortion via the local stretching ratio (STR) induced by the mapping from the spherical surface to the ERP plane. As shown in Fig. 1, assuming a spherical element $d\theta d\phi$ whose area is $\delta S(\theta, \phi)$. After ERP, the planar area element $dudv$ with a center point $(u, v)$ is defined as $\delta P(u, v)$. The differential relation between element $d\theta d\phi$ and $\delta P(u, v)$ is captured by the Jacobian determinant $dudv = J(\theta, \phi)d\theta d\phi$ as follows:

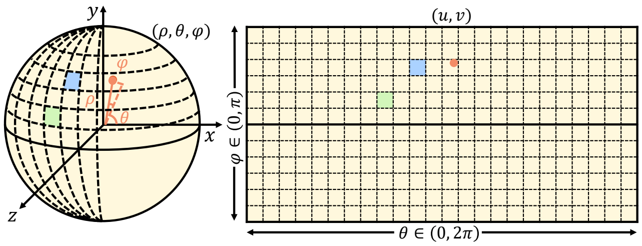


Figure 1: Geometric explanation of transforming between the ideal spherical surface and ERP plane.

$$J(\theta, \phi) = \frac{\partial(u, v)}{\partial(\theta, \phi)} = \begin{vmatrix} \frac{\partial(u)}{\partial(\theta)} & \frac{\partial(v)}{\partial(\phi)} \\ \frac{\partial(u)}{\partial(\theta)} & \frac{\partial(v)}{\partial(\phi)} \end{vmatrix}. \tag{3}$$

Furthermore, the area $\delta P(u, v)$ and $\delta S(\theta, \phi)$ are equal to $|dudv|$ and $d\theta d\phi\cos(\phi)$, respectively. Therefor, the area stretching ratio $\text{STR}(u, v)$ can be derived as:

$$\text{STR}(u, v) = \frac{\delta S(\theta, \phi)}{\delta P(u, v)} = \frac{|d\theta d\phi|\cos(\phi)}{|dudv|} = \frac{\cos(\phi)}{\left|\frac{\partial(u,v)}{\partial(\theta,\phi)}\right|} = \frac{\cos(\phi)}{|J(\theta, \phi)|}. \tag{4}$$

From Eq. 2, we can conclude that $|J(\theta, \phi)| = 1$, thus obtaining $\text{STR}(u, v) = \cos(\phi)$ for ERP. As a result, ERP distortions are fully characterized by latitudes. As latitude increases, STR decreases, and distortion becomes more severe. Therefore, we formulate STR as latitude-related pixel weights ranging from 0 to 1:

$$W_{lat}(u, v) = \cos((v - (H/2) + 0.5)\pi/H). \tag{5}$$

## 2. Experimental Results

As mentioned in the main paper, more comparisons of computational efficiency, visualization, spatio-temporal consistency, user study, and ablation study are provided in this section. To provide a thorough demonstration of the effectiveness of STDAN on the real-world ODV-SR task, we examine various aspects in practical application scenarios.

*Corresponding author.

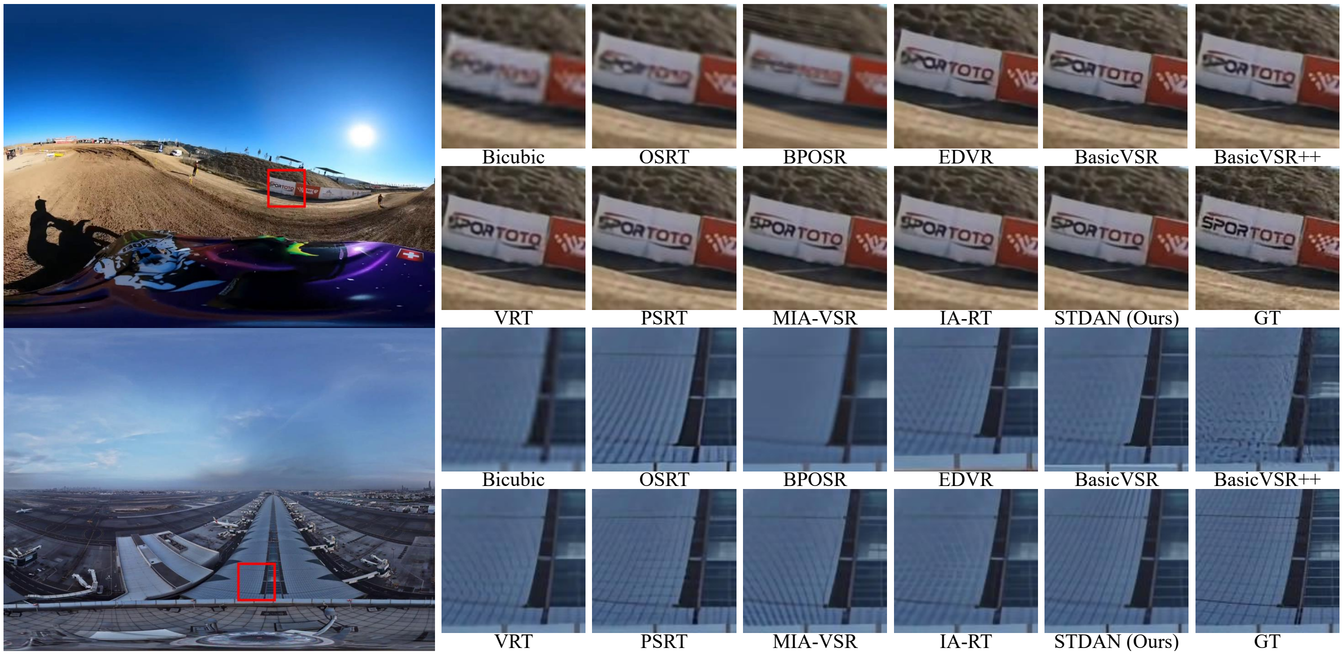


Figure 2: Qualitative ×4 ODV-SR comparison on ERP *ODV-SR* dataset.

| Method | OSRT | BPOSR | BasicVSR | BasicVSR++ | VRT | PSRT | MIA-VSR | IA-RT | STDAN(Ours) |
|---|---|---|---|---|---|---|---|---|---|
| Parameters(M) | 1.09 | 2.07 | 6.29 | 7.03 | 33.44 | 12.31 | 15.64 | 12.36 | 13.12 |
| FLOPs(T) | 0.1597 | 0.3507 | 0.8968 | 0.9619 | 3.2097 | 4.8029 | 2.8384 | 4.9163 | 1.8621 |
| Runtime(s) | 0.7243 | 0.4378 | 0.1859 | 0.2512 | 1.8507 | 4.6278 | 3.3991 | 5.4140 | 0.6960 |
| WS-PSNR(dB) | 28.11 | 28.41 | 29.64 | 29.83 | 30.06 | 30.14 | 30.17 | 30.18 | 30.23 |

Table 1: Computational efficiency comparison of ×4 ODV-SR on *ODV-SR* dataset.

**2.1 Computational Efficiency Comparison** The computational efficiency is evaluated and shown in Tab. 1. As the number of FLOPs(T) and Runtime(s) is related to the resolution of input video sequences, we therefore report the average per-frame results on the proposed *ODV-SR* dataset with the practical high-resolution (HR) need of ODVs. We also adopt this approach to facilitate fair comparison between single-frame ODI-SR methods (OSRT and BPOSR) and multi-frame models (BasicVSR, BasicVSR++, VRT, PSRT, MIA-VSR, and IA-RT). From Tab. 1, STDAN achieves a faster running speed and fewer FLOPs compared to SOTA Transformer-based VSR methods VRT, PSRT, MIA-VSR, and IA-RT, primarily due to the lightweight network architecture design. Meanwhile, STDAN performs best in the term of WS-PSNR by incorporating ODV-specified spatio-temporal modulation modules. Notably, compared to IA-RT, our STDAN has a similar model size but operates much faster with better reconstruction performance.

**2.2 Qualitative Comparison** We visualize more comparison results of different VSR methods in Fig. 2. In the first case, only STDAN restores the letters "S" without wrong branches. As for curved architectural texture structures, STDAN reconstructs continuous and consistent curves and matches the texture distribution in the GT image. Although PSRT generates a grid-like structure successfully, the lines within it are twisted and disconnected. More intuitively, STDAN clearly rebuilds the exact count of glass panes while SOTA MIA-VSR and IA-RT introduce superfluous white window dividers.

**2.3 Spatio-Temporal Consistency Comparison** As described in the main paper, we visualize temporal profiles of different algorithms in Fig. 3. The temporal profiles are obtained by stitching horizontal rows at the same location in consistent frames. It is observed that multi-frame based methods significantly outperform single-frame based approaches (Bicubic, BPOSR, and OSRT). Moreover, the reconstruction results of STDAN avoid over-smoothing and are closer to the ground truth.

**2.4 User Study** To intuitively compare the spatio-temporal quality of ODVs reconstructed by different methods, we perform a user study to select the better one from the results of STDAN and other approaches. In detail, we invite 15 participants to compare STDAN with BasicVSR++, VRT, PSRT, MIA-VSR, and IA-RT in pairs, respectively. As depicted in Fig. 5, volunteers prefer the performance of our STDAN.

**2.5 Ablation Study** As mentioned in the main paper, extensive ablation studies are conducted to demonstrate the ef-

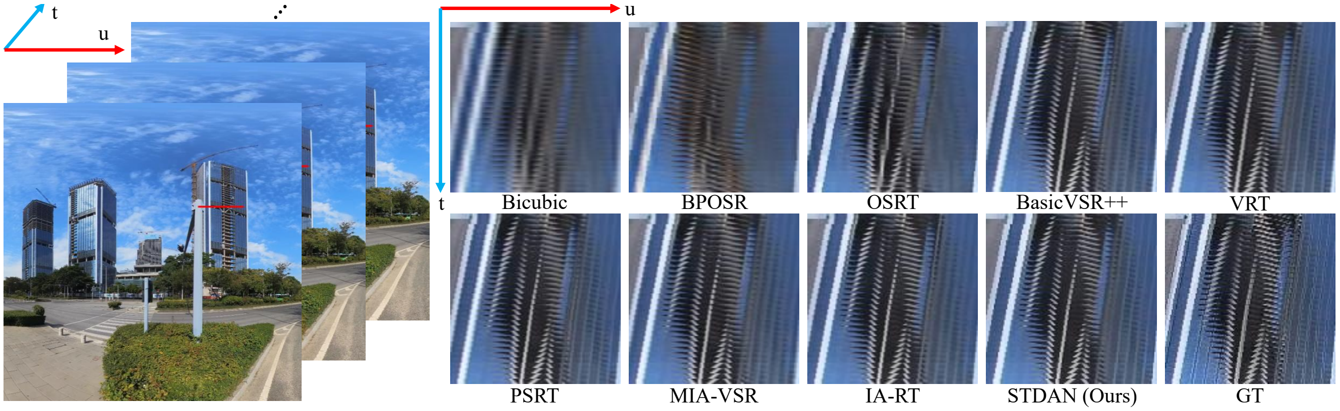


Figure 3: Temporal profile comparison of ×4 ODV-SR on ERP *ODV-SR* dataset.

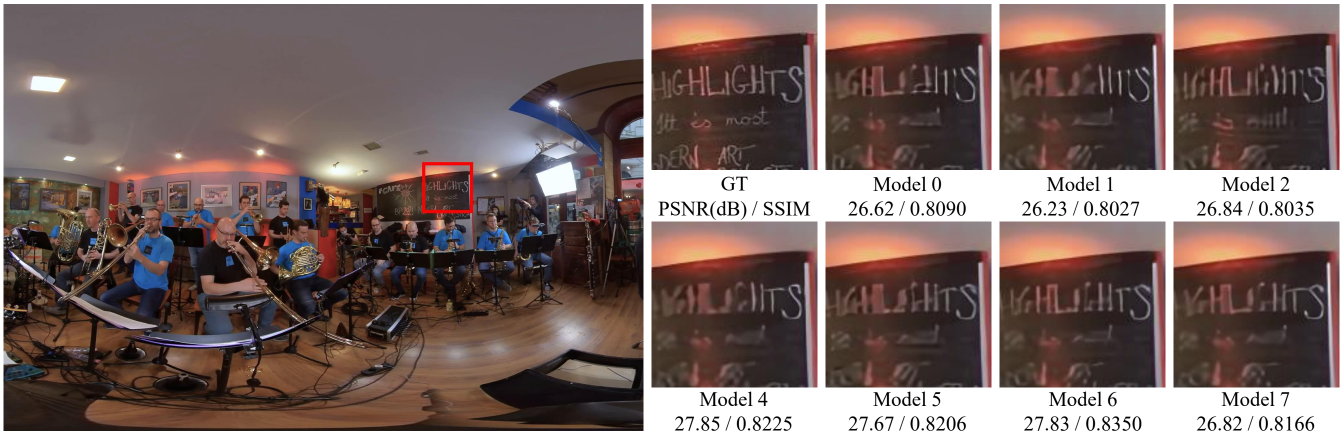


Figure 4: Subjective ablation study of ×4 ODV-SR with different modules on ODV-SR dataset. The PSNR and SSIM of the local regions are provided for a more intuitive comparison.

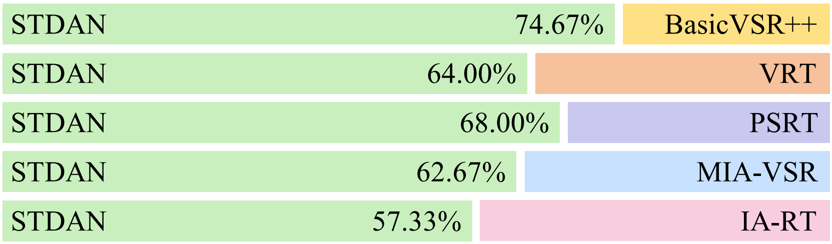


Figure 5: User study results of ×4 ODV-SR on *ODV-SR* dataset. The values represent the percentage of the participants preferring the results of STDAN compared with other methods.

fectiveness of the introduced spatio-temporal modules. Furthermore, we visualize ×4 ODV-SR results of models with proposed modules. As presented in Fig. 4, the improved models reconstruct sharper frames, especially Models 4, 5, 6, and 7, which successfully recover the letters "GHTS" that are blurred in the baseline Model 0. Compared with the baseline network, incorporating the proposed modules can produce more accurate texture details with a pleasing visual feeling. In terms of patch PSNR and SSIM, Model 1 degrades since it inclines to emphasize equator areas. Other models all make progress, and Model 6 has an obviously better SSIM, which improves the visual quality.

## References

Sun, Y.; Lu, A.; and Yu, L. 2017. Weighted-to-spherically-uniform quality evaluation for omnidirectional video. *IEEE signal processing letters*, 24(9): 1408–1412.
